# Supplementary material for: Interplay of transport mechanisms during the evaporation of a pinned sessile water droplet
Source: arXiv:2103.00132 ancillary file (2021-02-27)
Supplement: Supplementary file 1 [file Supplementary_Material.pdf]

Supplementary Material for

# Interplay of transport mechanisms during the evaporation of a pinned sessile water droplet

Osman Akdag[a], Yigit Akkus[a], Barbaros Çetin[b], Zafer Dursunkaya[c]

[a]ASELSAN Inc., 06200 Yenimahalle, Ankara, Turkey
[b]İ.D. Bilkent University, 06800 Çankaya, Ankara, Turkey
[c]Middle East Technical University, 06800 Çankaya, Ankara, Turkey

A. Simulations with open boundaries

B. Simulations for isothermal substrate

C. Near interface vapor concentration during Bénard-Marangoni instability

## A. Simulations with open boundaries

Physical boundaries of a problem determine the boundary conditions for the equations governing the problem. The effect of boundaries (boundary conditions) on the solution is simply known as the boundary effect. In the modeling of droplet evaporation into the air, a common practice is to include a very large gas volume (compared to the size of the droplet) with open boundaries in order to eliminate the boundary effect on the results. This approach is useful when the volume of the surrounding air is excessively large such that droplet evaporation has no observable effect at the outer air flow. However, if the gas volume is not sufficiently large, the outer flow can be affected by the evaporation of the droplet, which, in turn, influence the droplet evaporation. In such a case, real physical boundaries of the problem should be considered during the modeling.

In this study, physical boundaries of the environmental chamber are utilized in the modeling of the experiments carried out in [1]. However, previous modeling studies [2-4] utilized large gas volumes with open boundaries. To investigate the effect of boundary selection, additional simulations are carried out by using open boundaries for the same problem. At the substrate temperature of 55.4 °C, droplet lifetime is found 171 s, which is 3.5% larger than the solution with the boundaries of environmental chamber. In addition to the considerable deviation in droplet lifetime, global evaporation rate thereof, instant evaporation rates are found to be fluctuating during the drying stages. The reason of this fluctuation can be understood by examining the outer gas flows as shown in Fig. S1, where the flow field is demonstrated by pink streamlines at three selected consecutive contact angles. As seen in the figure, outer gas flow reveals different flow patterns. First (at θ=60°), two vortices form near the substrate. Then they merge and form a single vortex at θ=56°. Finally (at θ=52°), vortex structures disappear completely. As a result, evaporation rates fluctuates considerably. Compared to simulations with environmental chamber, instant evaporation rates deviate by 2.7%, 1.3%, and 5.3% at the contact angles of 60°, 56°, and 52°, respectively.

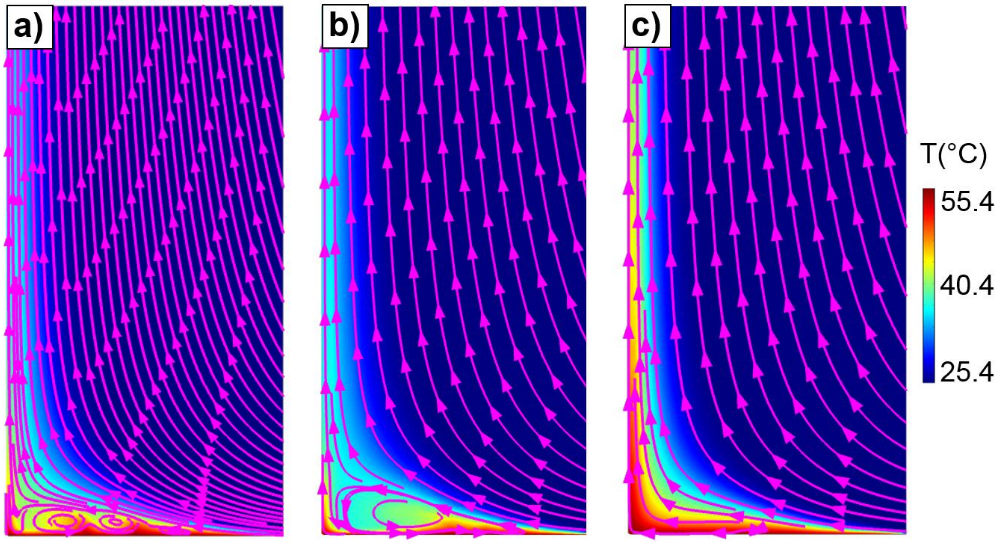


**Figure S1:** Temperature field and streamlines in the gas phase in the simulation with open boundaries for the droplet contact angles of **a)** 60°, **b)** 56°, and **c)** 52°. The substrate temperature is 55.4°C. Radius and height of the gas volume are 250 and 470 mm, respectively. Droplet is not observable due to its small scale (R=1.44 mm).

## B. Simulations for isothermal substrate

Resultant velocity and temperature fields together with the superimposed energy flux and velocity streamlines are reported for the isothermal substrate. When thermocapillarity is accounted for, a single large convection cell is created by the surface flow from the contact line to the apex, the direction of decreasing interface temperature. The orientation of this vortex structure is designated as CCW direction relying on the right side positioned images, which include streamlines in the droplet domain, in Fig. S2a. This CCW single vortex is present during the most of the droplet lifetime. At very small contact angles ($\theta < 4°$), on the other hand, radial flow replaces the Marangoni convection. It should be noted that Bénard -Marangoni instability does not occur in isothermal substrate case. When thermocapillarity is not accounted for, the interplay between buoyant and radial flows shapes the velocity field. At relatively higher contact angles, a large single Rayleigh convection cell is created by buoyant forces in CW direction as shown in Fig. S2b. Then radial flow starts to dominate the buoyancy-induced convection cell. Finally, radial flow damps the Rayleigh convection completely at the contact angle of 32°. After that, radial flow is effective till the dryout.

When Marangoni flow is effective, energy flux streamlines follow the velocity streamlines indicating the convection as the primary energy transport mode. In the absence of Marangoni flow, conduction is mainly responsible for the energy transport as demonstrated by non-stretched energy flux streamlines between the substrate and droplet surface.

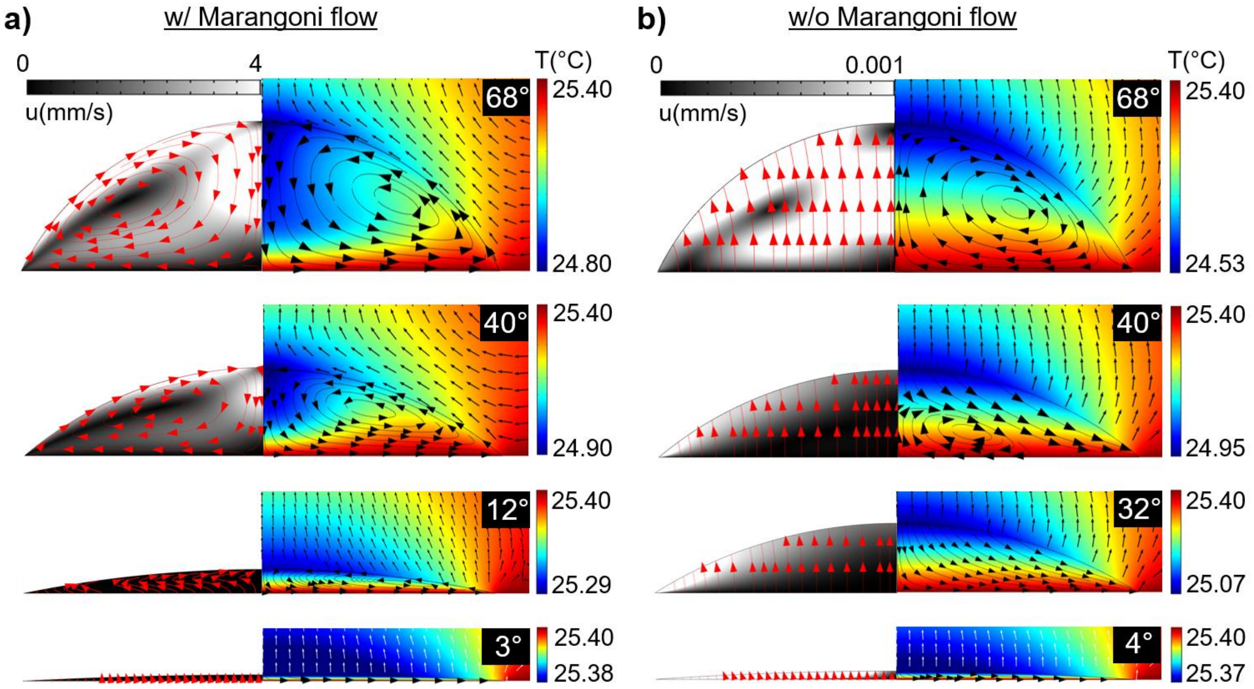


**Figure S2:** Velocity magnitude field (left images) inside the droplet with superimposed total energy flux streamlines and temperature field (right images) inside the droplet with superimposed velocity streamlines and in the near droplet gas region with superimposed normalized velocity vectors in the **a)** presence and **b)** absence of thermocapillarity. Substrate temperature is 25.4°C, same with the far field temperature. The value of the corresponding contact angle is

specified at each plot. Note that velocity magnitude scale bars in **a)** and **b)** are common for the corresponding plots, whereas individual temperature scale bars are utilized for each plot.

## C. Near interface vapor concentration during Bénard-Marangoni instability

In the presence of Bénard-Marangoni convection cells, evaporation dynamics is greatly affected by the associated interfacial velocity distribution. Consequently, the distribution of near interface vapor concentration is shaped by the evaporation and gas dynamics. Figure S3 shows near interface vapor concentration with Bénard-Marangoni instability at selected contact angles.

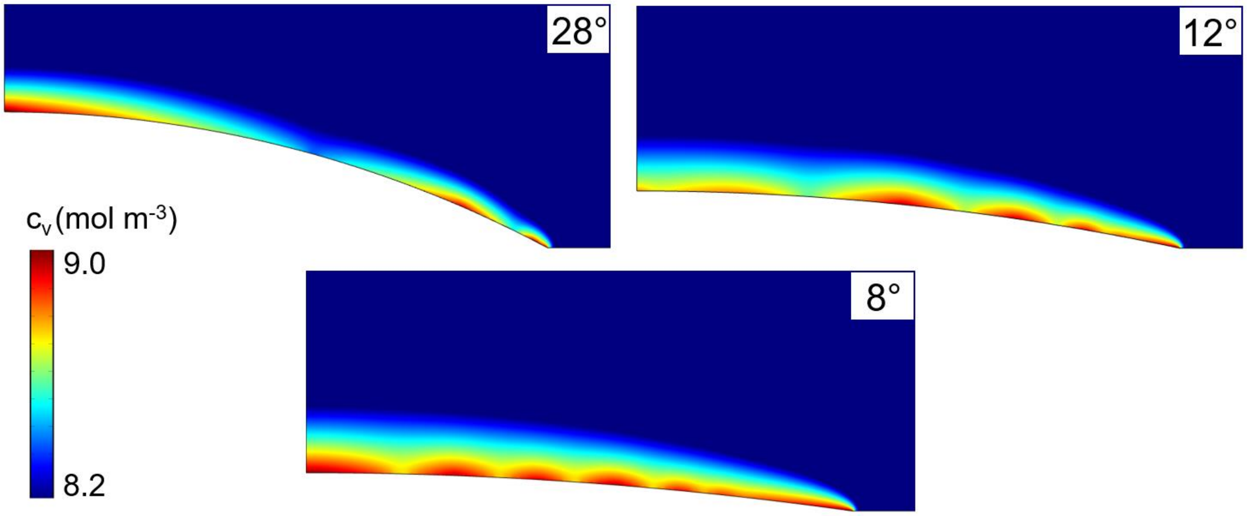


**Figure S3:** Near interface vapor concentration with Bénard-Marangoni instability for the contact angles 28°, 12°, and 8°. The substrate temperature is 65.4°C.


### References

[1] B. Sobac and D. Brutin. Thermal effects of the substrate on water droplet evaporation. *Phys. Rev. E,* 86(2):021602, 2012.

[2] Y. H. Chen, W. N. Hu, J. Wang, F. J. Hong, and P. Cheng. Transient effects and mass convection in sessile droplet evaporation: The role of liquid and substrate thermophysical properties. *Int. J. Heat Mass Tran.*, 108:2072-2087, 2017.

[3] M. Kumar and R. Bhardwaj. A combined computational and experimental investigation on evaporation of a sessile water droplet on a heated hydrophilic substrate. *Int. J. Heat Mass Tran.*, 122:1223-1238, 2018.

[4] Z. Pan, J. A. Weibel, and S. V. Garimella. Transport mechanisms during water droplet evaporation on heated substrates of different wettability. *Int. J. Heat Mass Tran.*, 152:119524, 2020.
